# Supplementary material for: Hide Your Malicious Goal Into Benign Narratives: Jailbreak Large Language Models through Carrier Articles
Source: arXiv:2408.11182 source file (2025-02-07)
Supplement: Supplementary file 1 [file appendix.tex]

\appendix
